# Supplementary material for: Generative Coarse-Graining of Molecular Conformations
Source: arXiv:2201.12176 source file (2022-06-16)
Supplement: Supplementary file 1 [file appendix.tex]

\label{appendix}

\subsection{coarse-graining and lifting operator of a toy example}
\label{app: toy-exampe}
Consider a cluster map $\map$ that cluster $\{1, 2, 3, 4\}$ into $\{\{1, 2, 3\}, \{4\}\}$. % Then the cluster map $\map$ is $\{1, 1, 1, 2\}$. 
If we assume the mapping is constructed as geometrical centers, i.e., the mapping weights are equal for each CG particle, then:
$   \proj = 
\begin{bmatrix}
1/3 & 1/3 & 1/3 & 0 \\
0 & 0 & 0 & 1 
\end{bmatrix} 
$
and 
$
    \lift = \begin{bmatrix}
1 & 0 \\
1 & 0 \\
1 & 0 \\
0 & 1 
\end{bmatrix}
$. 
We have
$ % \begin{equation*}
    \proj \lift = \begin{bmatrix}
1 & 0 \\
0 & 1 
\end{bmatrix}  
$ % \end{equation*}
and
$ %\begin{equation*}
    \lift \proj = \Pi_{n} = \begin{bmatrix}
1/3 & 1/3 & 1/3 & 0\\
1/3 & 1/3 & 1/3 & 0\\
1/3 & 1/3 & 1/3 & 0\\
0 & 0 & 0 & 1\\
\end{bmatrix}.  
$ %\end{equation*}

In the case where all atoms are mapped to exactly one coarse bead, the $\lift$ is exactly the Moore-Penrose psuedo-inverse of $\proj$. 

Note that definition \ref{def:cg} do \emph{not} require that $\proj_{I, i}  \neq  0 \; \textit{ } \forall i \in S_I = \{k \in [n] | \map(x_k) = X_I\} $. Intuitively, this means that some atoms do not contribute to any coarse bead. For example some coarse-grained simulations only simulate $\alpha$ carbons on the backbone. 

For the case where $\proj_{I, i} =  0$ for some $i$, $\lift$ operator defined is no longer the pseudo-inverse of $\proj$. For example, if we assign 0 weights to two of the nodes in $\proj$ induced by $\map$:
\begin{equation*}
    \proj = \begin{bmatrix}
0 & 1 & 0 & 0 \\
0 & 0 & 0 & 1 
\end{bmatrix} 
\end{equation*}
From our definition $\ref{def:lift}$, $\proj^{+}$ remains the same \chen{is that true?} but is not the psuedo-inverse of $\proj$.

\subsection{ELBO Derivation}
We derive equation \ref{eq:elbo} here:

\begin{equation}
\begin{aligned}
    \log p(x|X) &= \log \E_{ q_\phi(z | x, X) } \frac{ p(x| X) }{q_\phi(z | x, X)} \\
    &\geq \E_{ q_\phi(z | x, X) } \log \frac{ p(x|X) }{q_\phi(z | x, X)} \\
    &= \E_{q_\phi(z | x, X)} \log \frac{  p_\theta(x | X, z)p_\psi(z|X)}{q_\phi(z | x, X)} \\
    &= \underbrace{\E_{q_\phi(z | x, X)} \log p_\theta(x | X, z)}_{\text{Reconstruction}} + \underbrace{\E_{q_\phi(z | x, X)} \log \frac{ p_\psi(z|X) }{q_\phi(z| x, X)}}_{\text{KL Divergence}}
% \label{eq:elbo}
\end{aligned}
\end{equation}

\subsection{Proofs}
\chen{To serve reader better, we should also move all statements in the appendix.}
\chen{need to fix the property numbering}

\subsubsection{Proof of property \ref{property:composition}}

% \begin{property}
% $\proj \lift = \mI_N.  \textit{ When} f_{i}=1 \textit{ } \forall i \in [n], \lift \proj = \Pi_{n}. $ 
% \end{property}
% Recall \cref{property:composition}
\begin{proof}
Because each $i$ only maps to unqiue $I$ (property of $\map$) and $\proj_{I, i}$ is normalized (definition \ref{def:cg}), we have:
\begin{equation*}
    \sum_{i \in [n]} \proj_{I, i} \lift_{i, I'} =
\begin{cases}
    1, & \text{if } I = I' \\
    0,              & \text{if } I \neq I' 
\end{cases}
    = \delta_{II'}
\end{equation*}
\end{proof}

\subsubsection{Proof of property \ref{property:m-equivariance}}
\begin{property}
$\proj: \R^{n\times3} \rightarrow \R^{N\times3}$ is E(3) equivariant:
\begin{equation*}
   \rotate \proj(x) + g = \proj(\rotate x + g) 
\end{equation*}
\end{property}

\chen{need to be more concise.}
\begin{proof}
For each $I$, its coarse coordinate are generates by: $X_I = \sum_i \proj_{I, i} x_i$. When applying an orthogonal and translation operation to $x_i$:
\begin{equation*}
    \sum_i \proj_{I, i} (\rotate x_i + g_i) 
\end{equation*}
where $g_i=g$ is the same for all $i$. Because the normalization condition for $\proj_{I, i}$, $\sum_i \proj_{I, i} g_i = g$. Because $\rotate$ operates in $\R^3$ so that it can be taken out of the summation, so we have: 
\begin{equation*}
    \sum_i \proj_{I, i} (\rotate x_i + g_i) = \rotate (\sum_i \proj_{I, i} x_i) + g = X_I + g 
\end{equation*}
Following from the definition of E(3) equivariance, we have shown that $\proj$ is equivariant. 
\end{proof}

\subsubsection{Proof of proposition \ref{prop:m-compat}}
\chen{need to discuss about the $\map (x)$ vs. $\map x$.}

\begin{proposition}
For any invariant features $z_1, z_2\in \mathbb{R}^F$, if $z_1 \neq z_2$ and $\dec(X,z_1) \neq \dec(X, z_2)$, then $\dec(X, z_1) \neq R(\dec(X, z_2))+g$ for any $R$ and $g$.
\label{prop:rotation_uniqueness}
\end{proposition}

\begin{proof}
    From linearity of $\proj$ and the property that $\proj \lift$ = I, we have 
    \begin{equation*}
    \begin{aligned}
        \proj(\dec(x,z)) &= \proj \lift X + \proj \Delta \tilde{x} - \proj \lift\proj(\Delta \tilde{x}) \\
                     &= X +  \proj \Delta \tilde{x} -\proj(\Delta \tilde{x})\\
                      &= X
    \end{aligned}
    \end{equation*}
\end{proof}

\subsection{Baseline method}

\textbf{Linear decoder} The linear projection baseline reconstructs from linear combinations of the coarse coordinates with learnable matrix $\mC$ as the coefficients.
\begin{equation*}
    \tilde{x}_{i, m} = f(X) = \sum_I C_{i, I} X_{I, m}
\end{equation*}
$m$ is the index for the Cartesian dimension. The set of coefficients are obtained by minimizing the Mean-Square Error between $\tilde{x}$ and $x$.
\begin{equation*}
    \mC = \argmin_{\mC} \frac{1}{3n } \sum_{m = 0 }^3 \sum_i (\tilde{x}_{i,m} - x_{i,m})^2
\end{equation*}
\wujie{visually compare samples from baseline methods}

\textbf{Equivariant linear decoder}

\subsection{Training and Model hyperparameters}

We use the hyperparameter set described in table \ref{tab:hyperparam} for the experiments we presented in the main text. The same set of hyperparameters are used for all choices of $N$.
\begin{table}[H]
\centering
\caption{hyperparameters used in the experiment. }
\label{tab:hyperparam}

\begin{tabular}{l|ll}
\toprule
                                                                        & Alanine Dipeptide & Chignolin \\ \midrule
\begin{tabular}[c]{@{}l@{}}encoder conv depth\end{tabular}           & 4                 & 2         \\
\begin{tabular}[c]{@{}l@{}}decoder conv depth\end{tabular}           & 6                 & 5         \\
\begin{tabular}[c]{@{}l@{}}all atom radius graph cutoff \chen{what is this?}\end{tabular} & 7.5               & 8.5       \\
\begin{tabular}[c]{@{}l@{}}CG radius graph cutoff\end{tabular}       & 11.0              & 20.0      \\
$F$ \chen{what is this?}                                                                       & 400               & 512       \\
\begin{tabular}[c]{@{}l@{}}batch  size\end{tabular}                   & 32                & 2         \\
\begin{tabular}[c]{@{}l@{}}learning  rate\end{tabular}                & 1e-4              & 9e-5      \\
\begin{tabular}[c]{@{}l@{}}activation  function\end{tabular}          & LeakyReLU         & swish     \\
\begin{tabular}[c]{@{}l@{}}training epochs\end{tabular}               & 250               & 50        \\
$\beta$                                                                  & 0.005             & 0.005   \\ \bottomrule 
\end{tabular}
\end{table}

\subsection{Mapping Generation protocols}

We introduce our mapping generation protocol implemented in our experiment. 

\textbf{Alanine Dipeptide} Given $N$, the cluster map $\map$ is randomly generated by randomly assigning each atom a value in $[0, N-1]$. We discard $m$ that does not cover cover $[0, N-1]$ to ensure that each alloted CG bead are assigned with at least one atom. 

\textbf{Chinolin} Because Chignolin is a large bio-molecule, we initialize $\map$ with the Girvan-Newman \chen{update this?} Algorithm to ensure that atoms that are close to each other are grouped together. The algorithm coarsens the graph by successively removing edges with high betweenness to cluster more connected nodes together. 

After initializing the mapping with Givan-Newman algorithm, We then randomly choose  $25\%$ of the atom and shuffle their assignment to create randomness in the generated mapping.

\subsection{More discussion about M-compatible decoders}

We illustrate the $\proj$-compatibility condition in figure \ref{fig:decode-compat}. We show that different choices of $z \sim p(z|X) $ can result in equivalent configurations with rotation and translation. Such degeneracy can be removed if we enforce the $\proj$-compatibility constraint. 

\begin{proposition}
For any invariant features $z_1, z_2\in \mathbb{R}^F$, if $z_1 \neq z_2$ and $\dec(X,z_1) \neq \dec(X, z_2)$, then $\dec(X, z_1) \neq R(\dec(X, z_2))+g$ for any $R$ and $g$.
\label{prop:rotation_uniqueness}
\end{proposition}

\begin{proof}

We apply proof with contradiction, by assuming the opposite of the statement to be true.

We apply M on the decoded coordinates generated by z1, and end up with the following contradiction: 
\begin{equation}
    	\proj(\dec(X, z_1)) = \proj(R \dec(X, z_2) + g)  = RX + g \neq \proj(\dec(X, z_1)) = X
\end{equation}

\end{proof}

This shows that the $z$-space does not encode E (3) actions, because its rotation and translation states are completely encoded by X, and the fine-grained coordinates depend on X.

\begin{figure*}
\centering
\includegraphics[width=\textwidth]{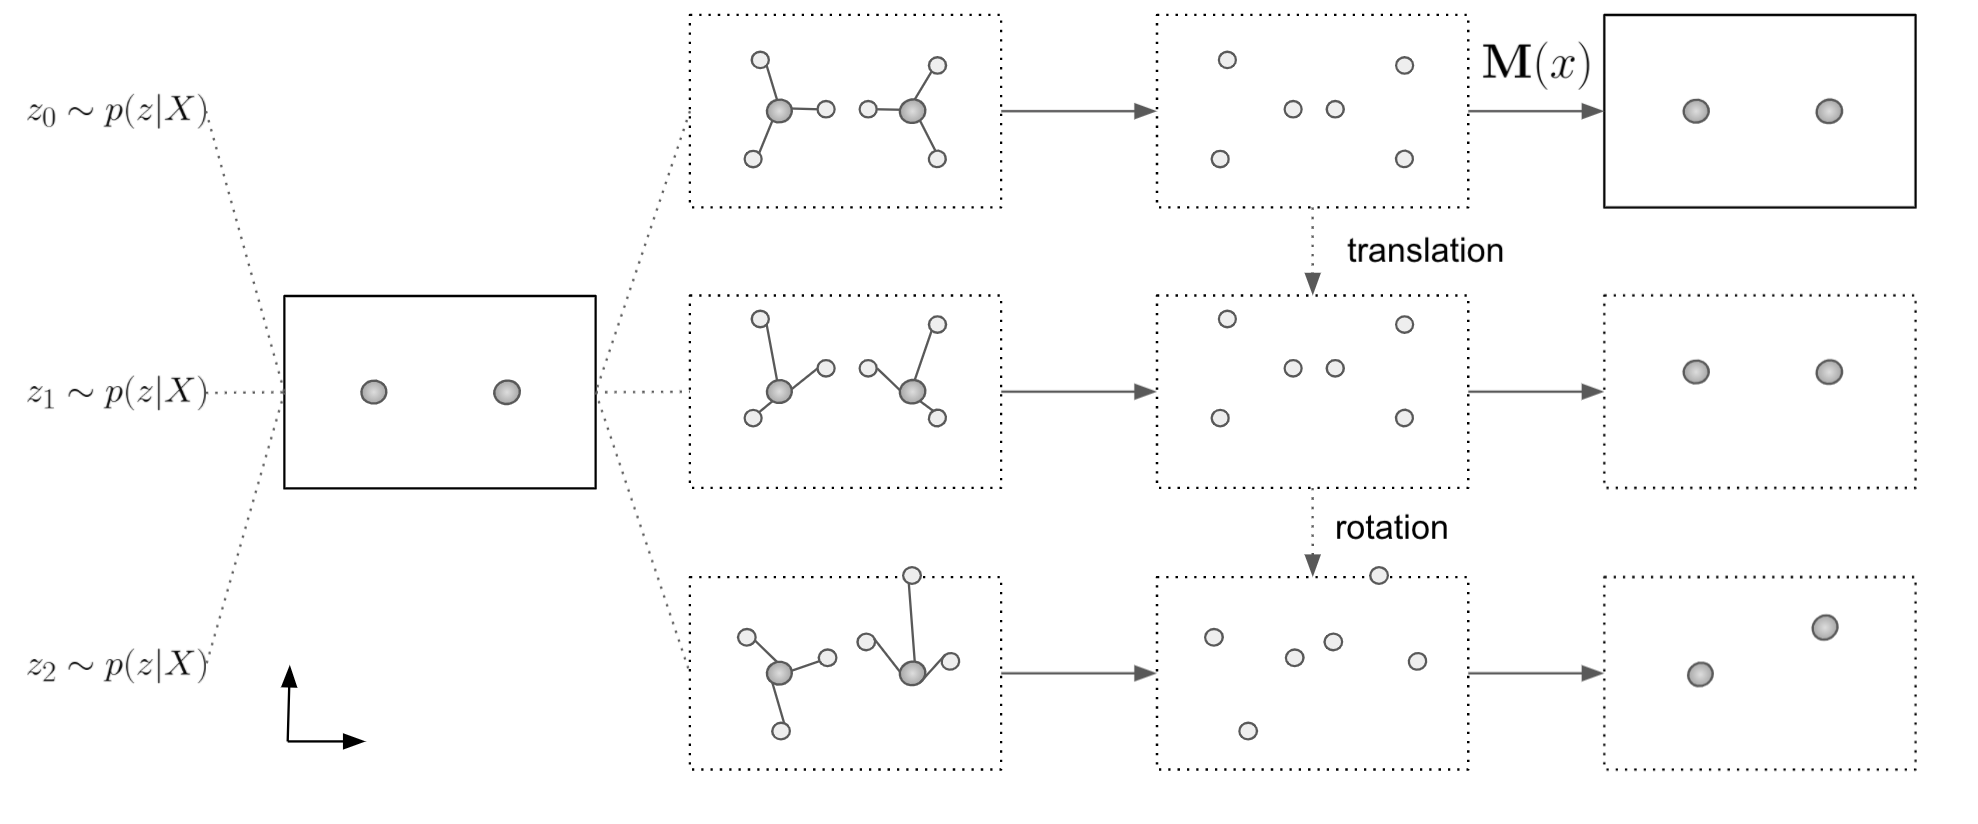}
\caption{Illustrating the need to constrain the compatibility between the decoded coordinates and CG coordinates }
\label{fig:decode-compat}
\end{figure*}

\section{More Results}

We show tabulated benchmark results in table \ref{tab:dipep_benchmark} and (?). CGVAE performs better in all cases. We also show samples of decoded geometries from baseline methods.

\begin{table}[]
\small
\centering
\caption{Tabulated model performances for our proposed model and the beaseline method.}

\begin{tabular}{llccccccc}
\toprule
\multirow{2}{*}{Metric}                                               & \multirow{2}{*}{Model} & \multicolumn{7}{c}{$N$}                 \\
                                                          &            & 3   & 4   & 5   & 6   & 8   & 10  & 12  \\ \midrule
                                                          
\multicolumn{1}{l|}{\multirow{2}{*}{\begin{tabular}[c]{@{}c@{}}
$\mathbf{RMSD}_{recon.}$ (heavy) \end{tabular}}}  & Linear Proj.      & 0.941 & 0.812 & 0.483 & 0.384 & 0.296 & 0.127 & 0.148 \\
\multicolumn{1}{l|}{}                                                & CGVAE         & 0.21 & 0.115 & 0.145 & 0.110 & 0.080 & 0.068 & 0.063 \\ \midrule

\multicolumn{1}{l|}{\multirow{2}{*}{\begin{tabular}[c]{@{}c@{}}
$\mathbf{RMSD}_{recon.}$ (all atom)\end{tabular}}} & Linear Proj.      & 1.125 & 1.022 & 0.585 & 0.541 & 0.439 & 0.361 & 0.275 \\
\multicolumn{1}{l|}{}                                                & CGVAE         & 0.530 & 0.128 & 0.160 & 0.119 & 0.090 & 0.080 & 0.071 \\ \midrule

\multicolumn{1}{l|}{\multirow{2}{*}{\begin{tabular}[c]{@{}c@{}}
$\mathbf{RMSD}_{gen.}$ (heavy)\end{tabular}}}  & Linear Proj.      & -   & -   & -   & -   & -   & -   & -   \\
\multicolumn{1}{l|}{}                                                & CGVAE         & 0.213 & 0.198 & 0.146 & 0.108 & 0.058 & 0.043 & 0.039 \\ \midrule

\multicolumn{1}{l|}{\multirow{2}{*}{\begin{tabular}[c]{@{}c@{}}
$\mathbf{RMSD}_{gen.}$ (all atom)\end{tabular}}} & Linear Proj.      & -   & -   & -   & -   & -   & -   & -   \\
\multicolumn{1}{l|}{}                                                & CGVAE         & 0.427 & 0.282 & 0.193 & 0.125 & 0.074 & 0.061 & 0.044 \\ \midrule

\multicolumn{1}{l|}{\multirow{2}{*}{\begin{tabular}[c]{@{}c@{}}
$\lambda$ (heavy)\end{tabular}}}          			& Linear Proj.      & 1.22 & 0.99 & 0.410 & 0.195 & 0.123 & 0.010 & 0.037 \\
\multicolumn{1}{l|}{}                                                & CGVAE         & 0.002 & 0.002 & 0.001 & 0   & 0   & 0   & 0   \\ \midrule

\multicolumn{1}{l|}{\multirow{2}{*}{\begin{tabular}[c]{@{}c@{}}
$\lambda$ (all atom)\end{tabular}}}        		    & Linear Proj.      & 1.501 & 1.339 & 0.519 & 0.322 & 0.267 & 0.199 & 0.044 \\
\multicolumn{1}{l|}{}                                                & CGVAE         & 0.042 & 0.01 & 0.01 & 0.004 & 0.005 & 0.001 & 0   \\ 
\bottomrule

\end{tabular}
\label{tab:dipep_benchmark}
\end{table}

% \subsection{On permutational equivariance of the decoded output} 

% We denote that the decode takes an unordered set of coarsened nodes as input, with each coarsened cluster represent a set of ordered set of nodes which the coarsened node includes. The decoder operates on the coarsened node set, with each coarsened node maps a set of fine-grained ordered node sets: 

% \begin{equation}
% \begin{Bmatrix}
% S_1 \\           
% \vdots \\
% S_I\\
% \vdots \\
% S_N
% \end{Bmatrix}  =
% \begin{Bmatrix}
% ( s_{1, 1}, ..., s_{1, k}, ..., s_{1, |S_1|} ) \\           
% \vdots \\
% ( s_{I, 1}, ..., s_{I, k}, ...,  s_{1, |S_I|} )\\
% \vdots \\
% ( s_{N, 1}, ..., s_{N, k}, ..., s_{1, |S_N|} )
% \end{Bmatrix} 
% \end{equation}

% In another word, specific vector channel correspond to specific fine-grained node for the decoder. The atomistic coordinates in the data are also ordered, so sorting is not required when estimating the reconstruction loss. Our model requires that the coarsened node set are defined consistently in the dataset and it is common to have consistent mapping choice for chemical modeling of macro molecules for macromolecules like proteins and heteropolymers.
